# Supplementary material for: GeLLMO: Generalizing Large Language Models for Multi-property Molecule Optimization
Source: arXiv:2502.13398 source file (2025-05-27)
Supplement: Supplementary file 1 [file BDQ_case1_appendix.tex]

\begin{figure}[htbp]
    \centering
    % First Case
    \begin{minipage}{0.43\linewidth}
        \centering
        \tiny $M_x$
        \includegraphics[width=1.0\linewidth]{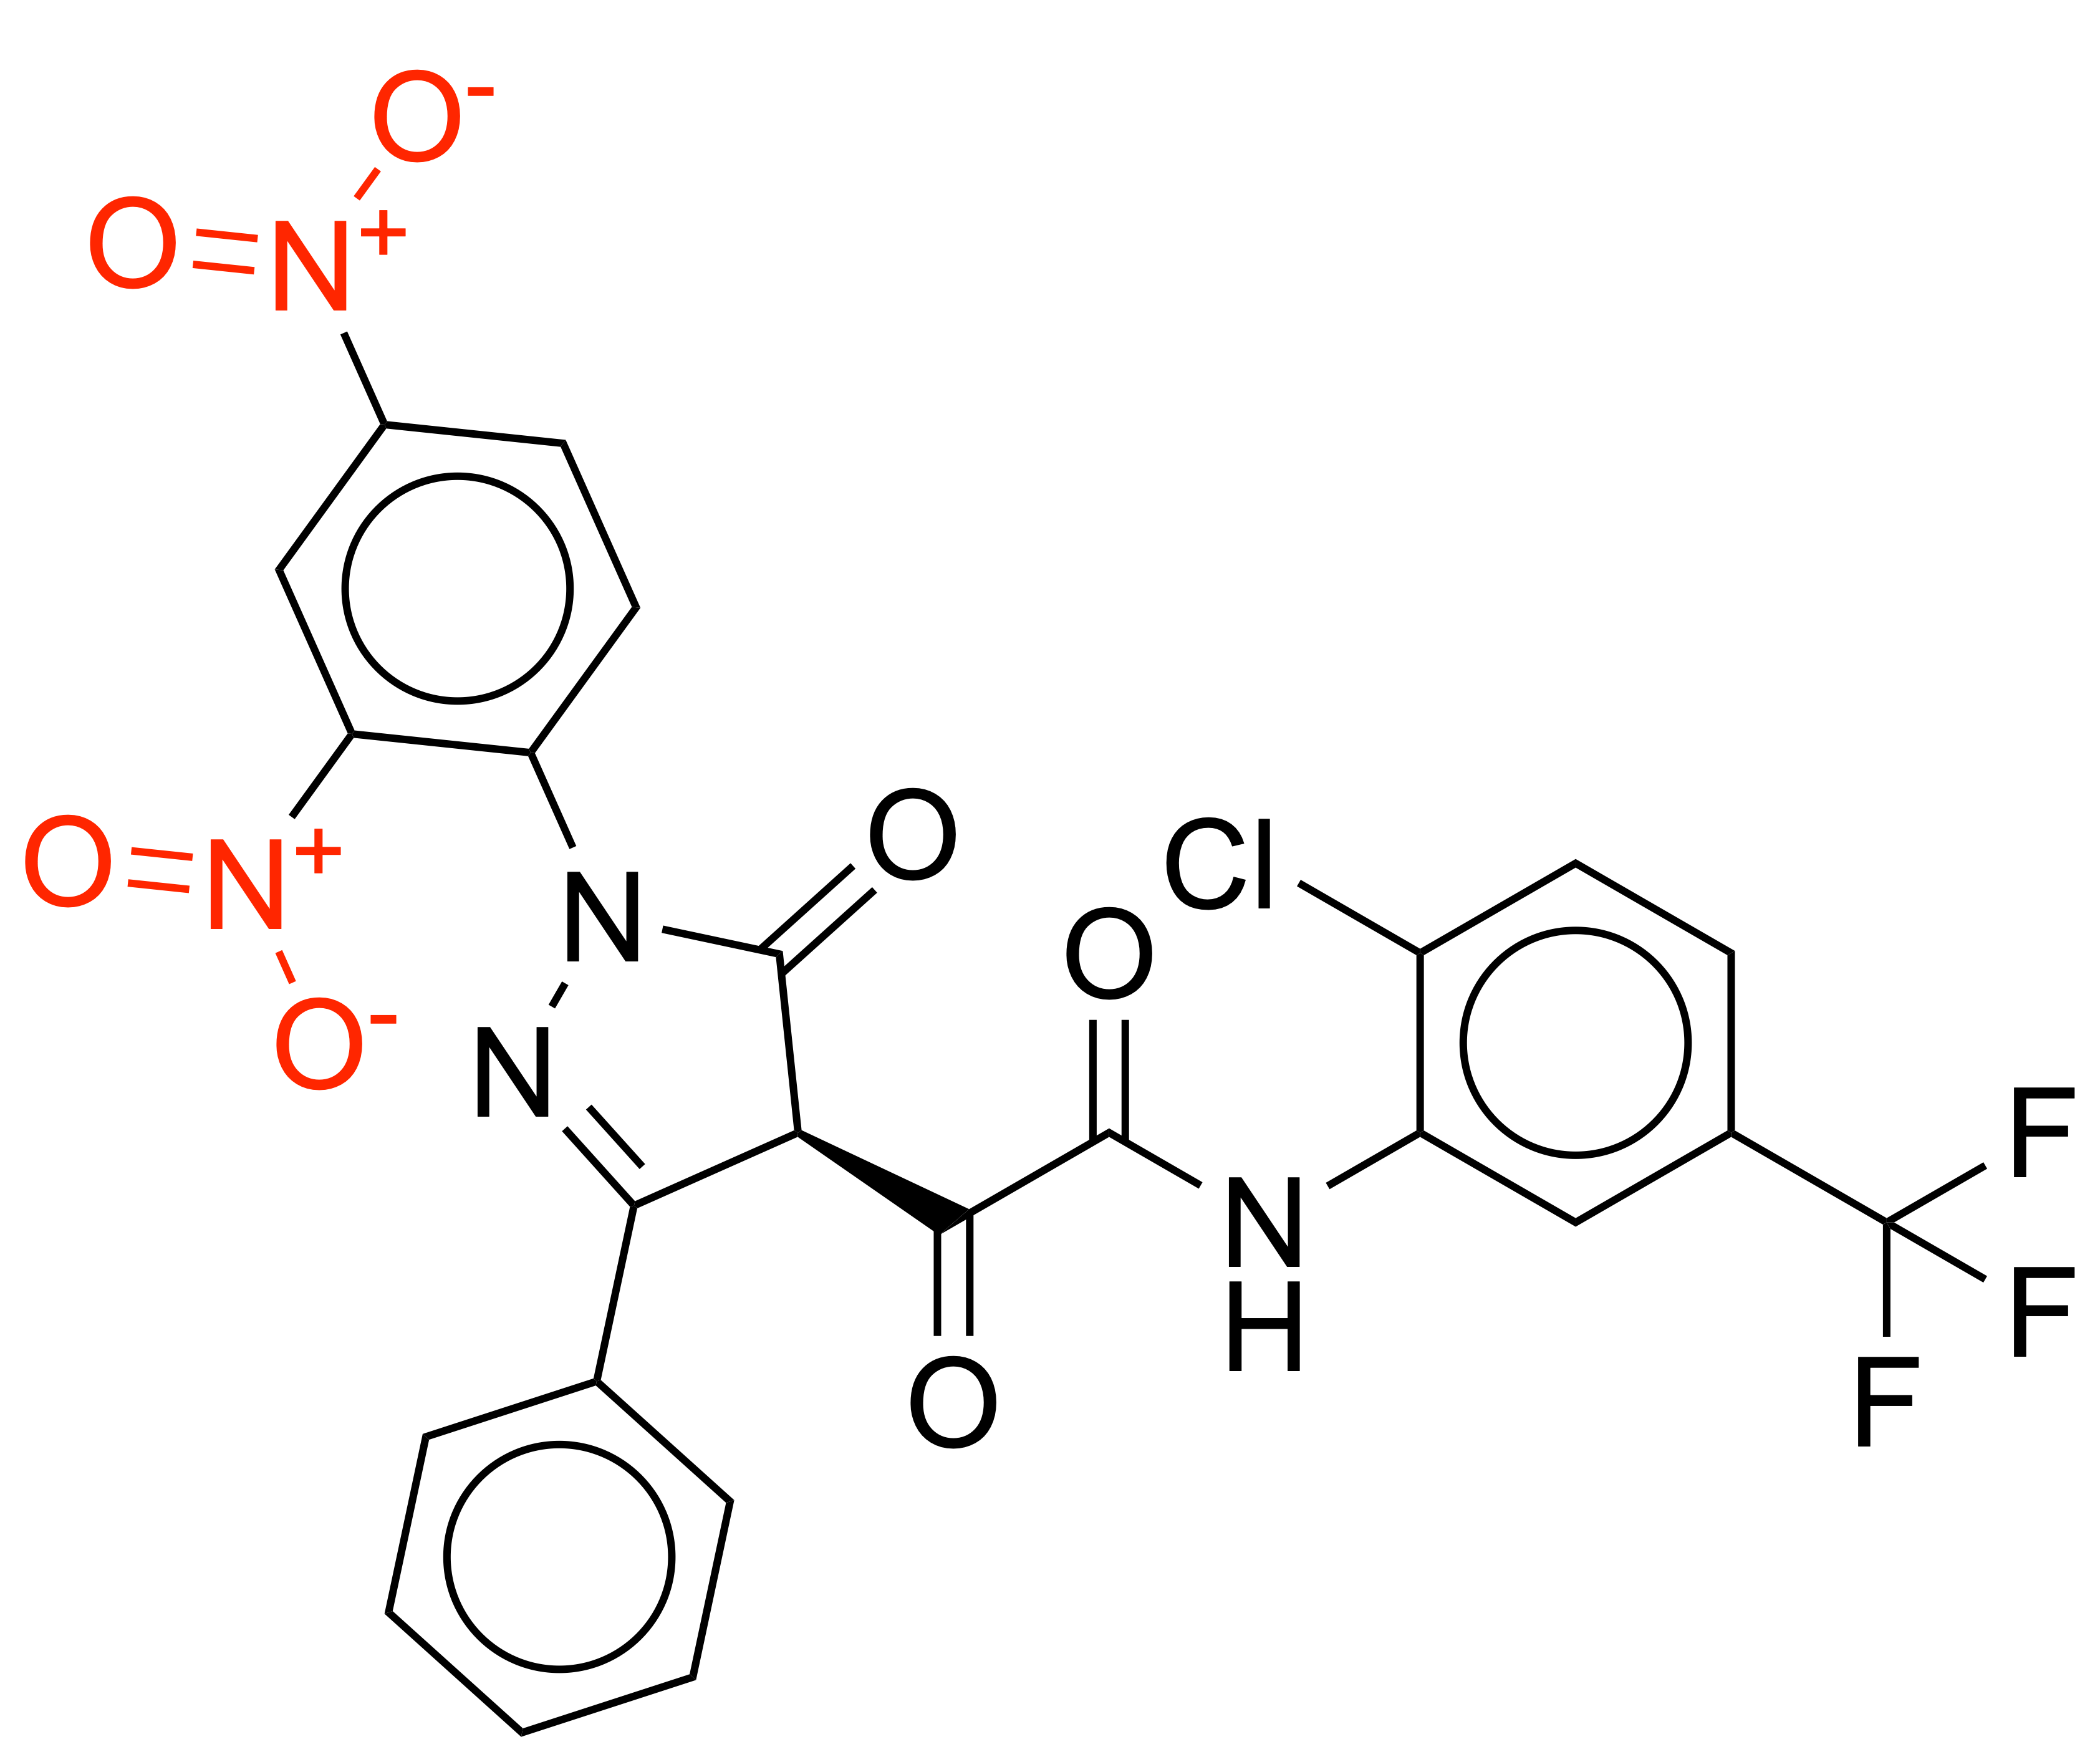}
        \par\vspace{2pt}
        \tiny BBBP=0.48, DRD2=0.00, \\
        \tiny QED=0.18
    \end{minipage}
    \hfill
    \begin{minipage}{0.1\linewidth}
        \centering \Large$\Rightarrow$\\
        \raggedright \tiny \mollm
        \raggedright \tiny \Sim=0.72
    \end{minipage}
    \hfill
    \begin{minipage}{0.44\linewidth}
        \centering
        \tiny $M_y$
        \includegraphics[width=1.0\linewidth]{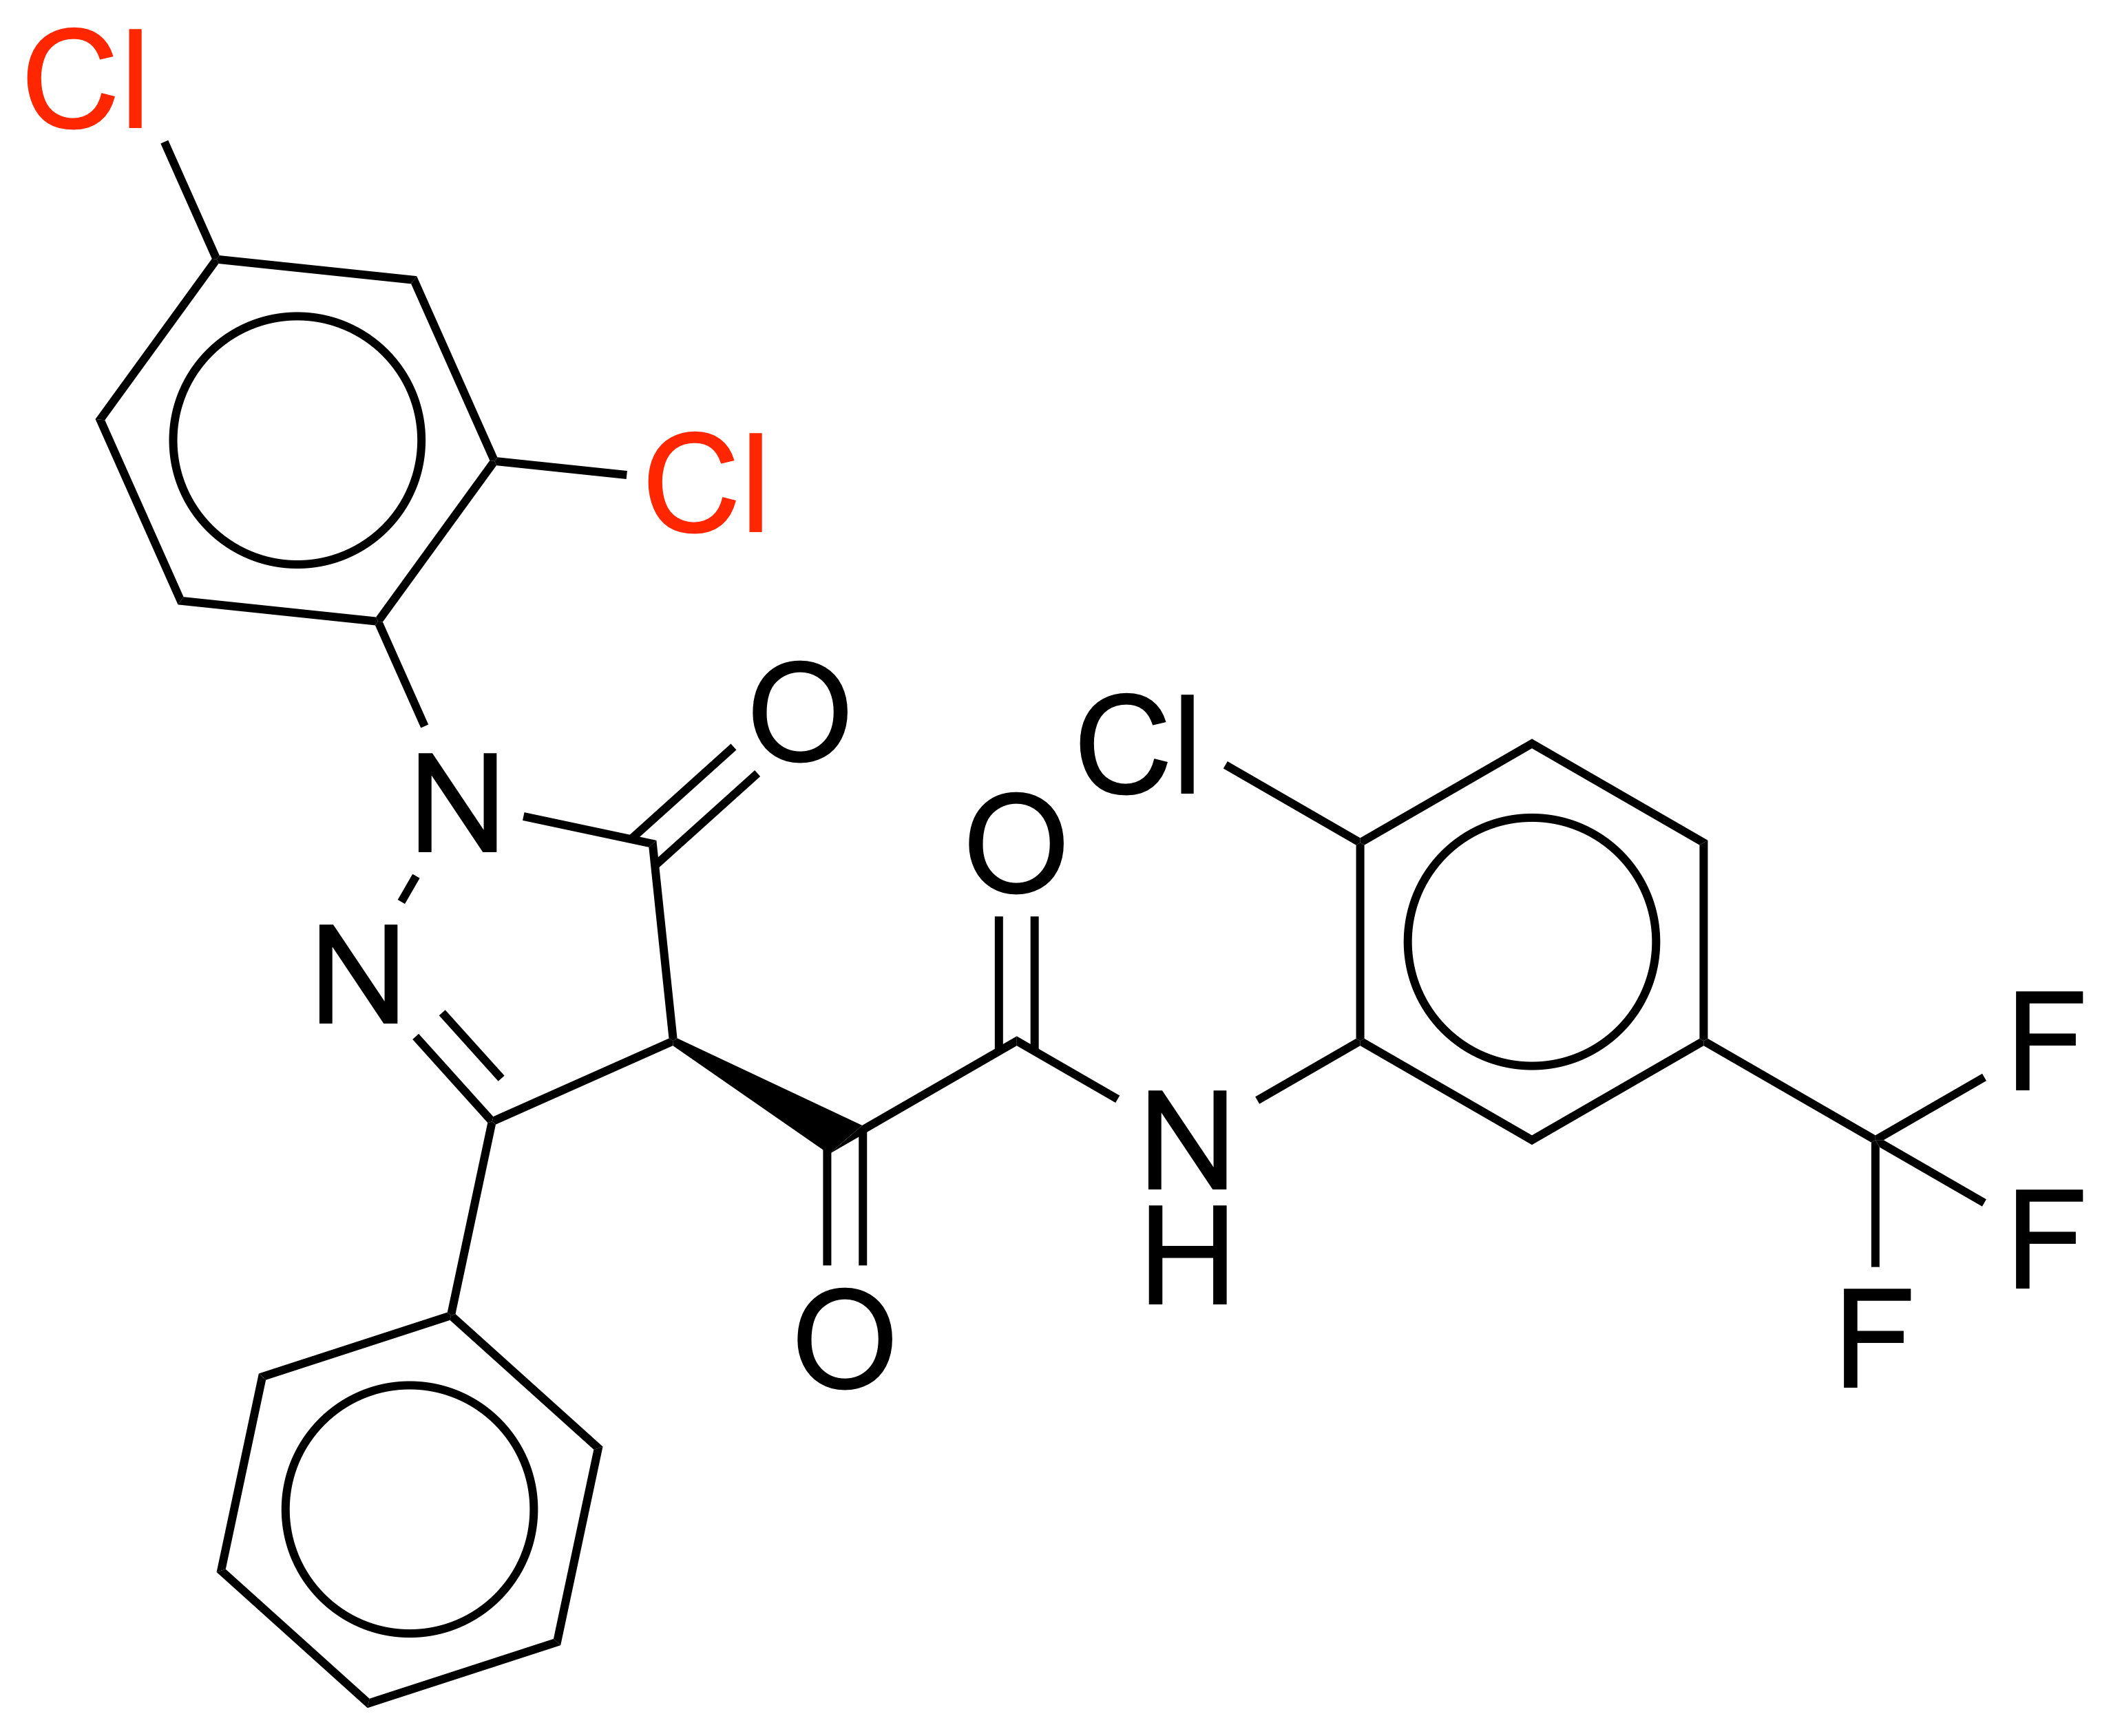}
        \par\vspace{2pt}
        \tiny BBBP=0.79 (+0.31),\\ 
        \tiny DRD2=0.01 (+0.01), QED=0.30 (+0.12)
    \end{minipage}

    \vspace{1em}

    % Second Case
    \begin{minipage}{0.43\linewidth}
        \centering
        \tiny $M_x$
        \includegraphics[width=1.0\linewidth]{./figures/BDQ_case1_mollm_src.png}
        \par\vspace{2pt}
        \tiny BBBP=0.48, \\
        \tiny DRD2=0.00, QED=0.18
    \end{minipage}
    \hfill
    \begin{minipage}{0.1\linewidth}
        \centering \Large$\Rightarrow$\\
        \raggedright \tiny \LlaSMol
        \raggedright \tiny \Sim=0.62
    \end{minipage}
    \hfill
    \begin{minipage}{0.44\linewidth}
        \centering
        \tiny $M_y$\\
        \includegraphics[width=1.0\linewidth]{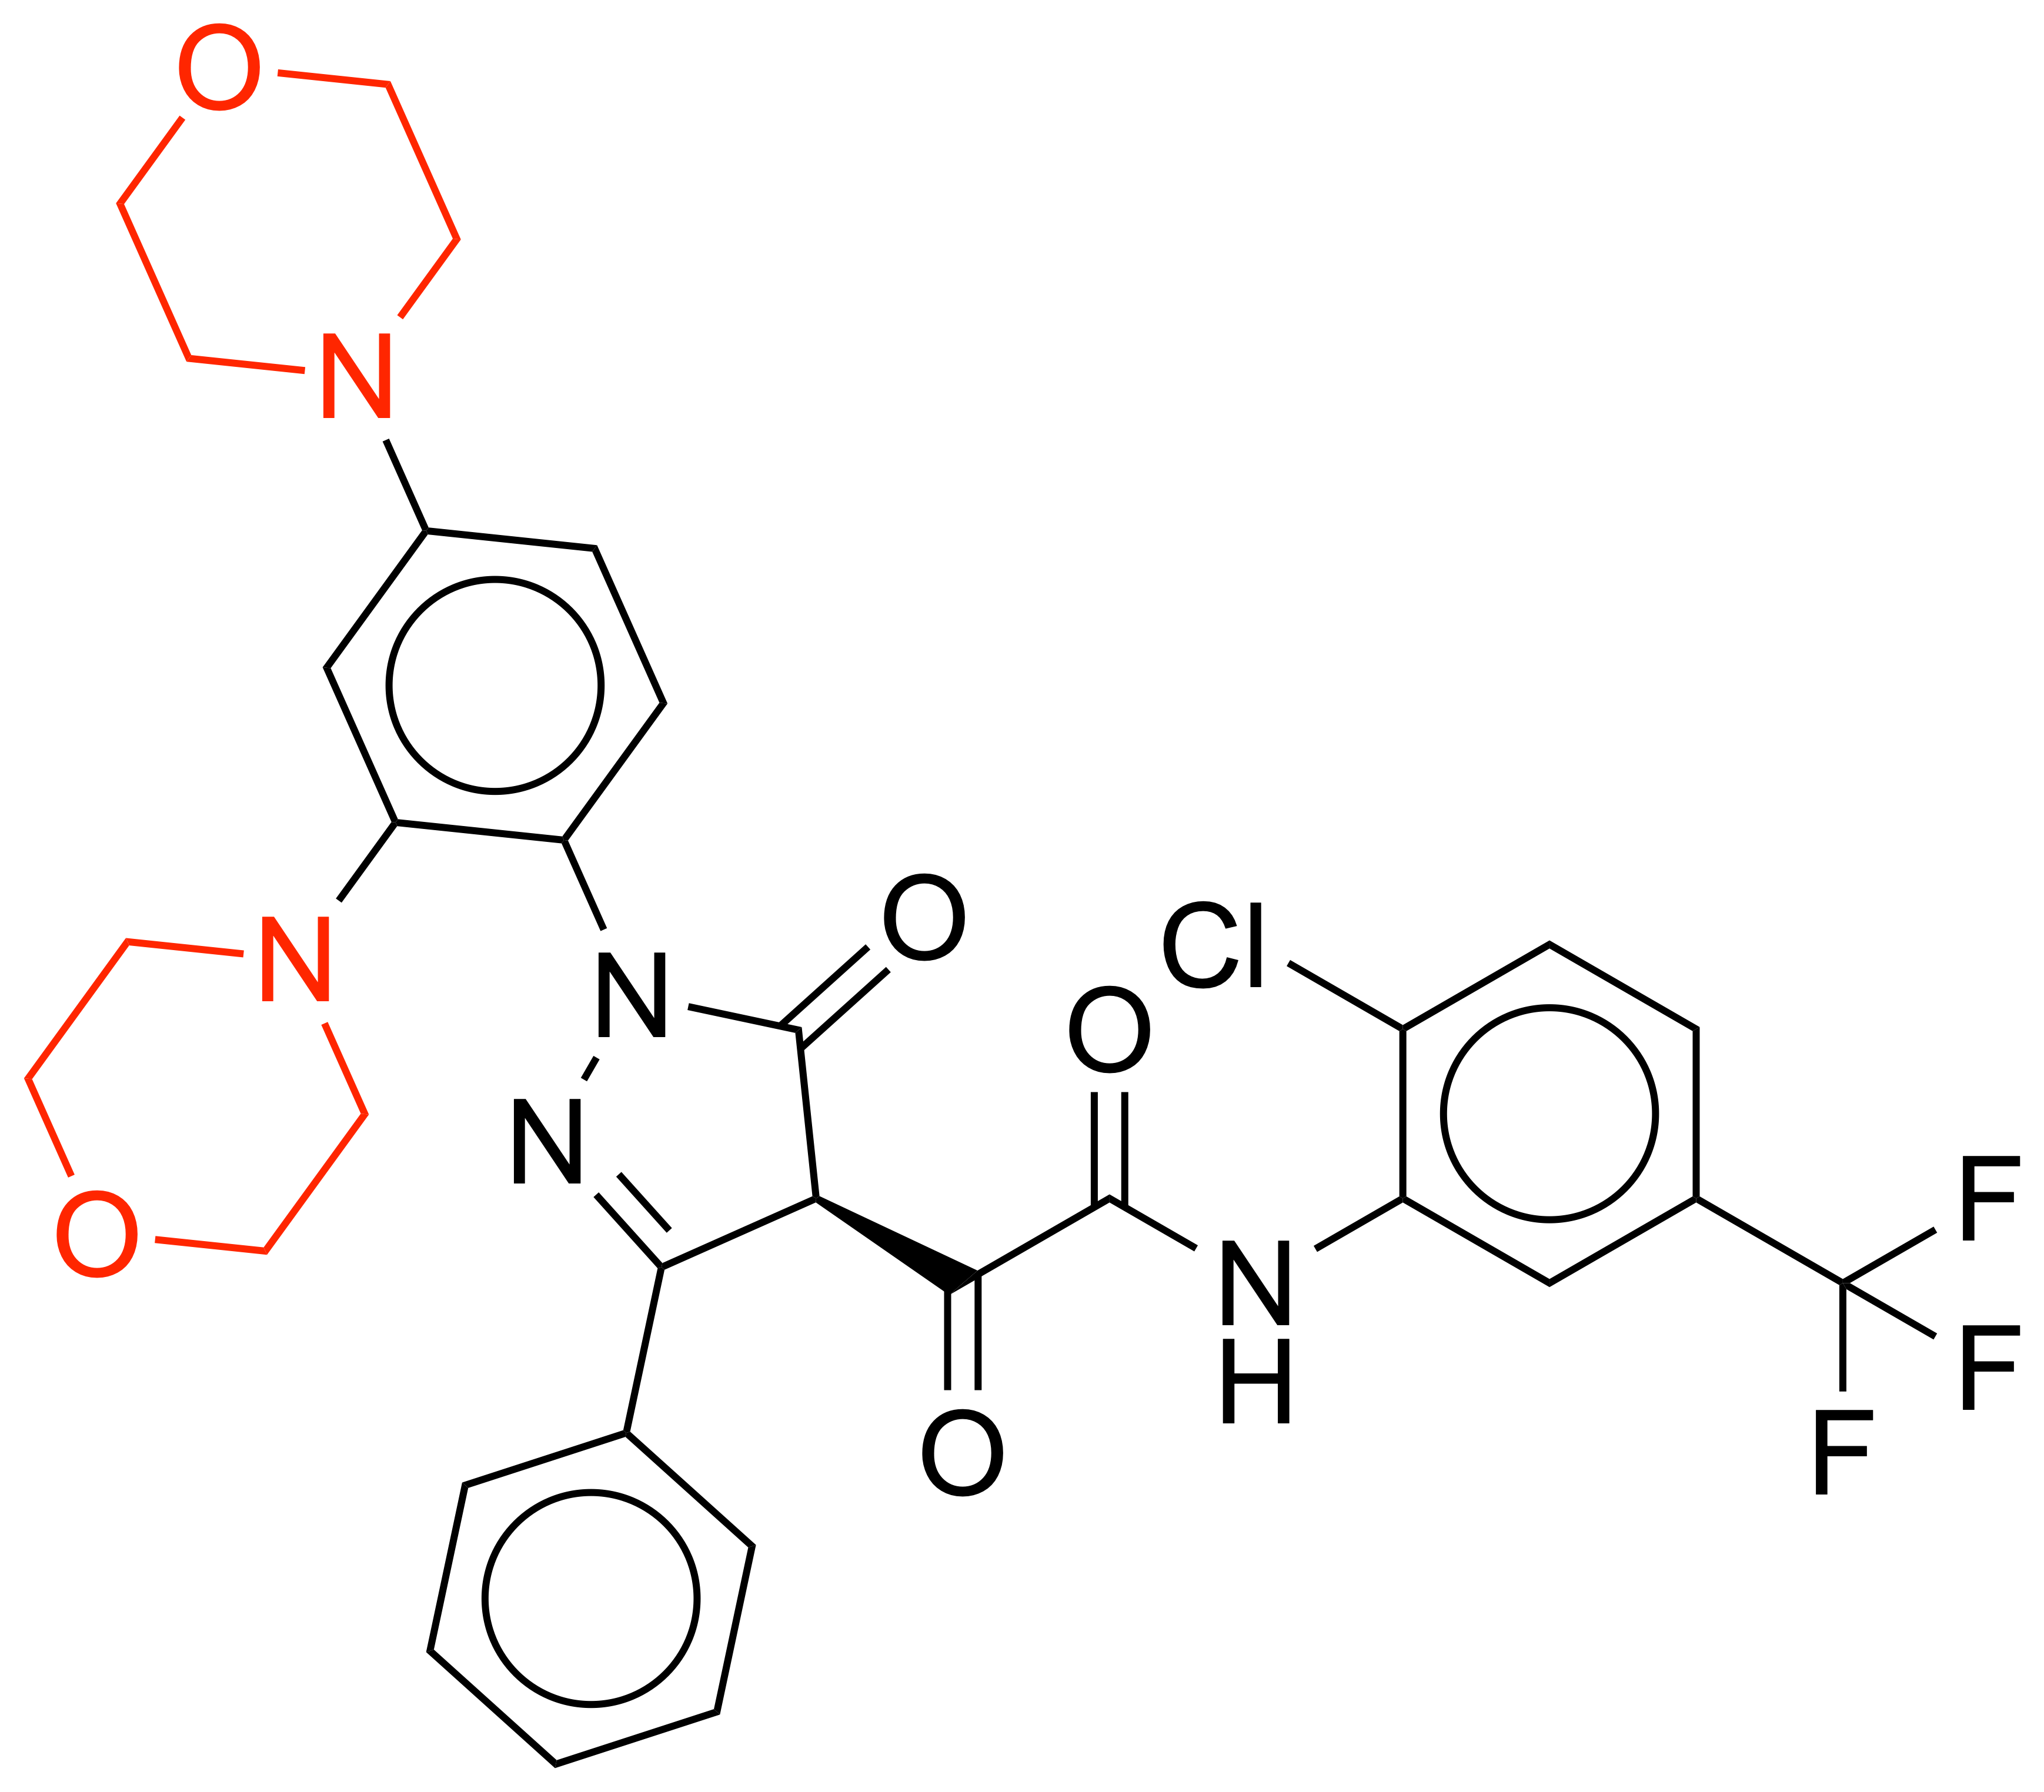}
        \par\vspace{1pt}
        \tiny BBBP=0.56 (+0.08), \\ 
        \tiny DRD2=0.03 (+0.03), QED=0.29 (+0.11)
    \end{minipage}
    %\caption{{\mollmSixGenM} and {\LlaSMolM}'s optimization cases on \BDQ. Modifications are highlighted in red.}
    %\label{fig:BDQ_case1_appendix}
\end{figure}
