# Supplementary material for: GeLLMO: Generalizing Large Language Models for Multi-property Molecule Optimization
Source: arXiv:2502.13398 source file (2025-05-27)
Supplement: Supplementary file 2 [file BDQ_case2_appendix.tex]

\begin{figure}[htbp]
    \centering
    % First Case
    \begin{minipage}{0.43\linewidth}
        \centering
        \tiny $M_x$
        \includegraphics[width=1.0\linewidth]{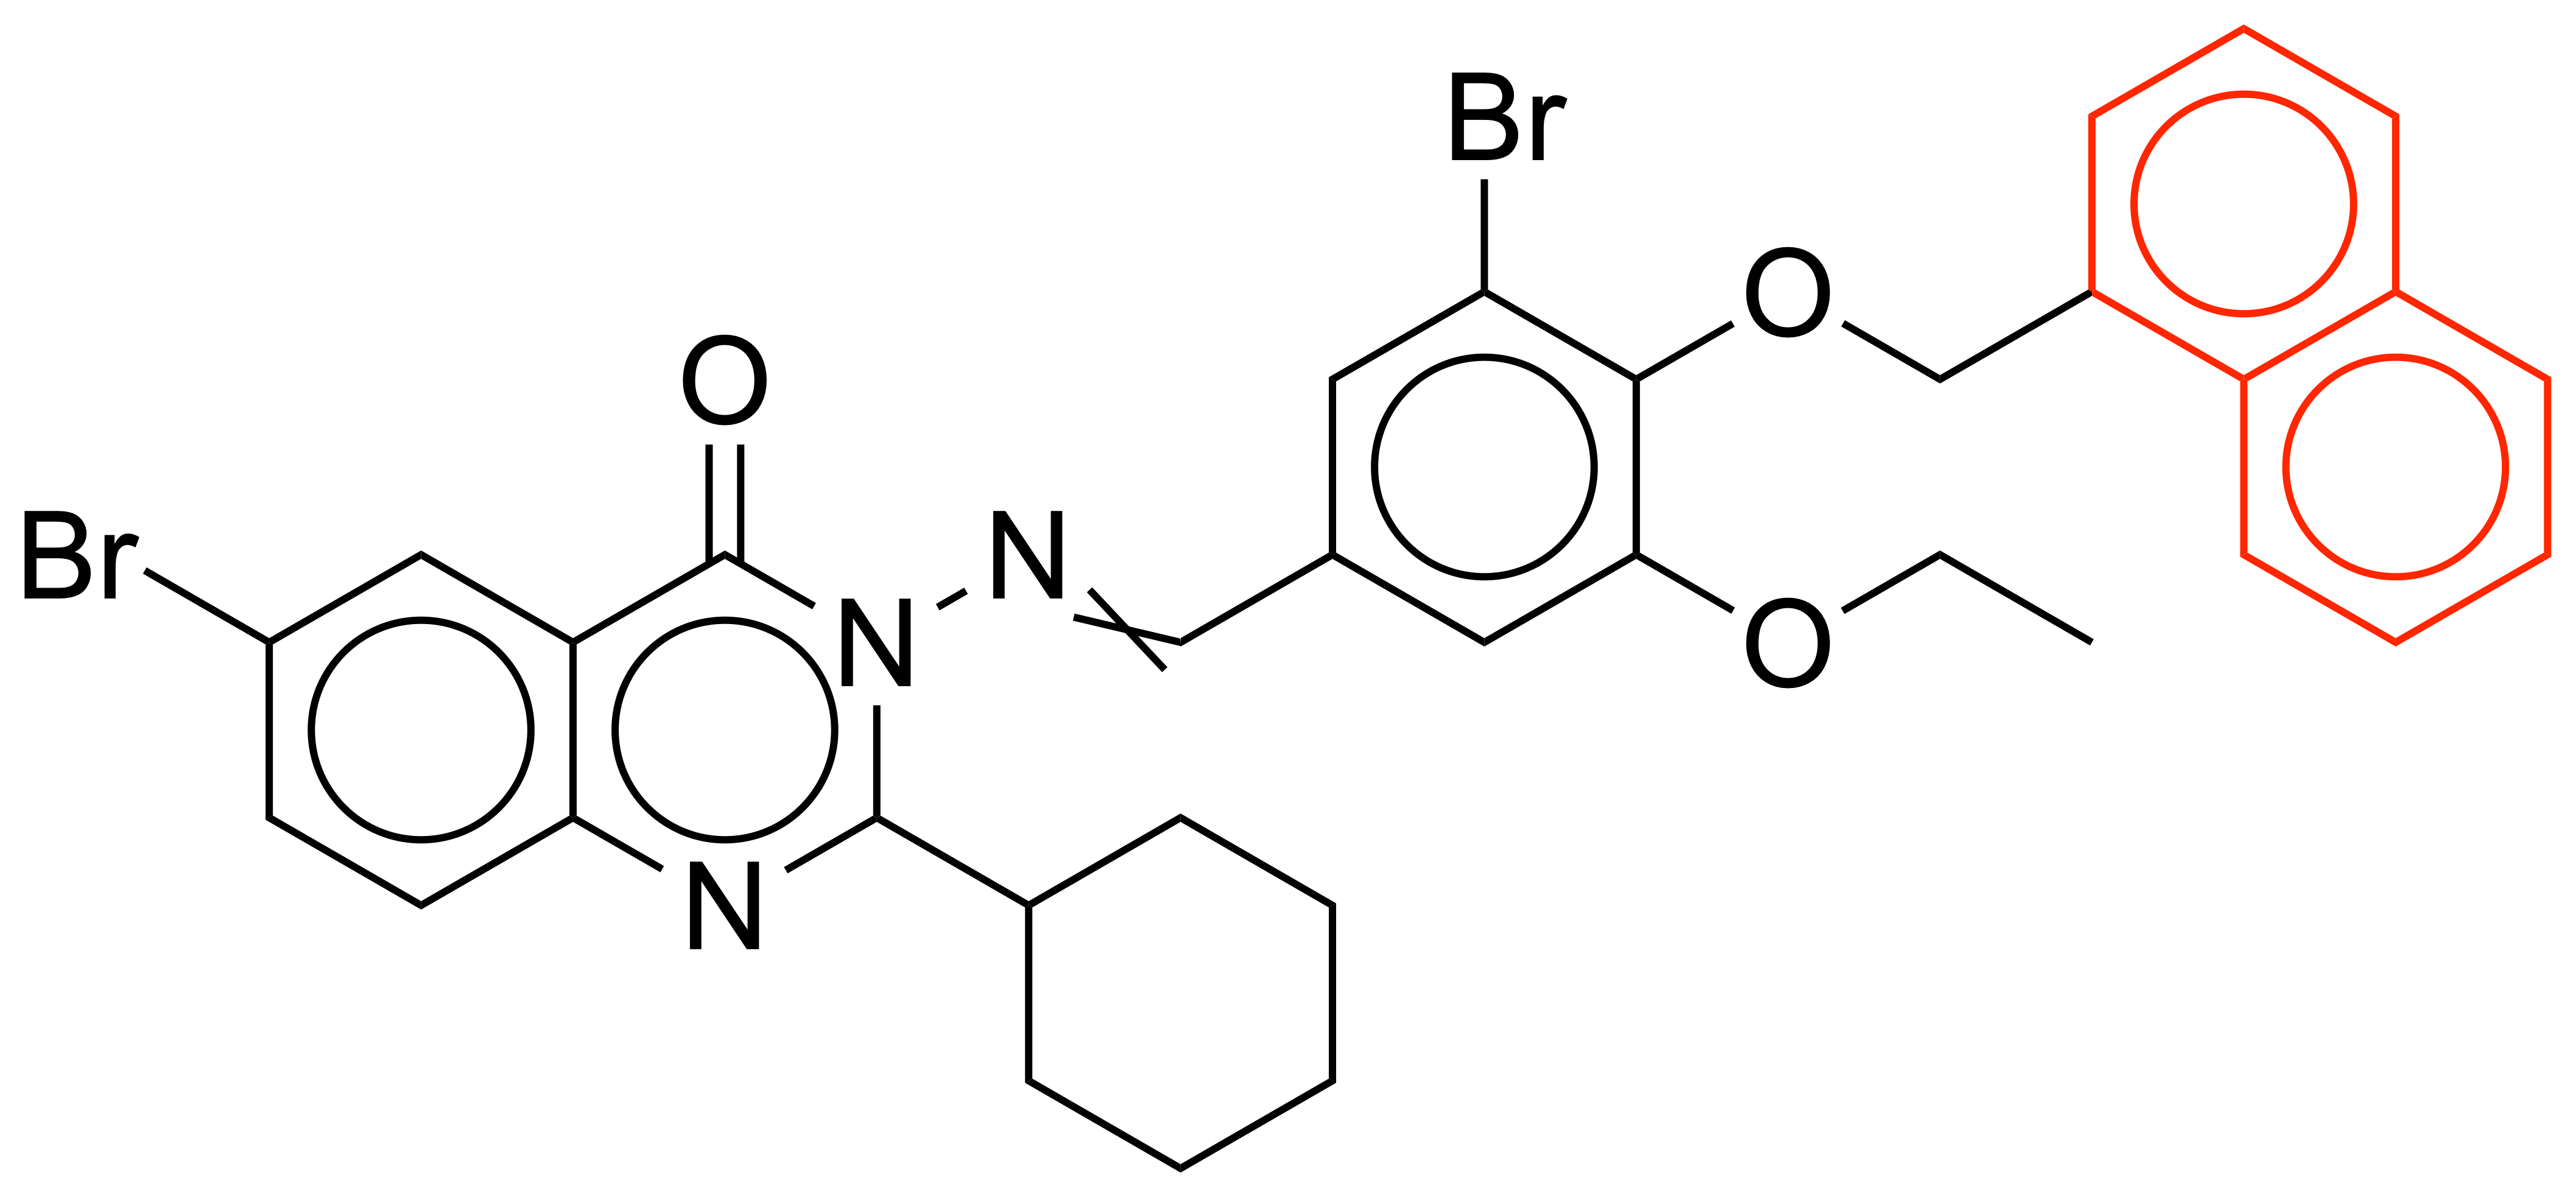}
        \par\vspace{2pt}
        \tiny BBBP=0.51, DRD2=0.06, \\
        \tiny QED=0.15
    \end{minipage}
    \hfill
    \begin{minipage}{0.1\linewidth}
        \centering \Large$\Rightarrow$\\
        \raggedright \tiny \mollm
        \raggedright \tiny \Sim=0.71
    \end{minipage}
    \hfill
    \begin{minipage}{0.44\linewidth}
        \centering
        \tiny $M_y$
        \includegraphics[width=1.0\linewidth]{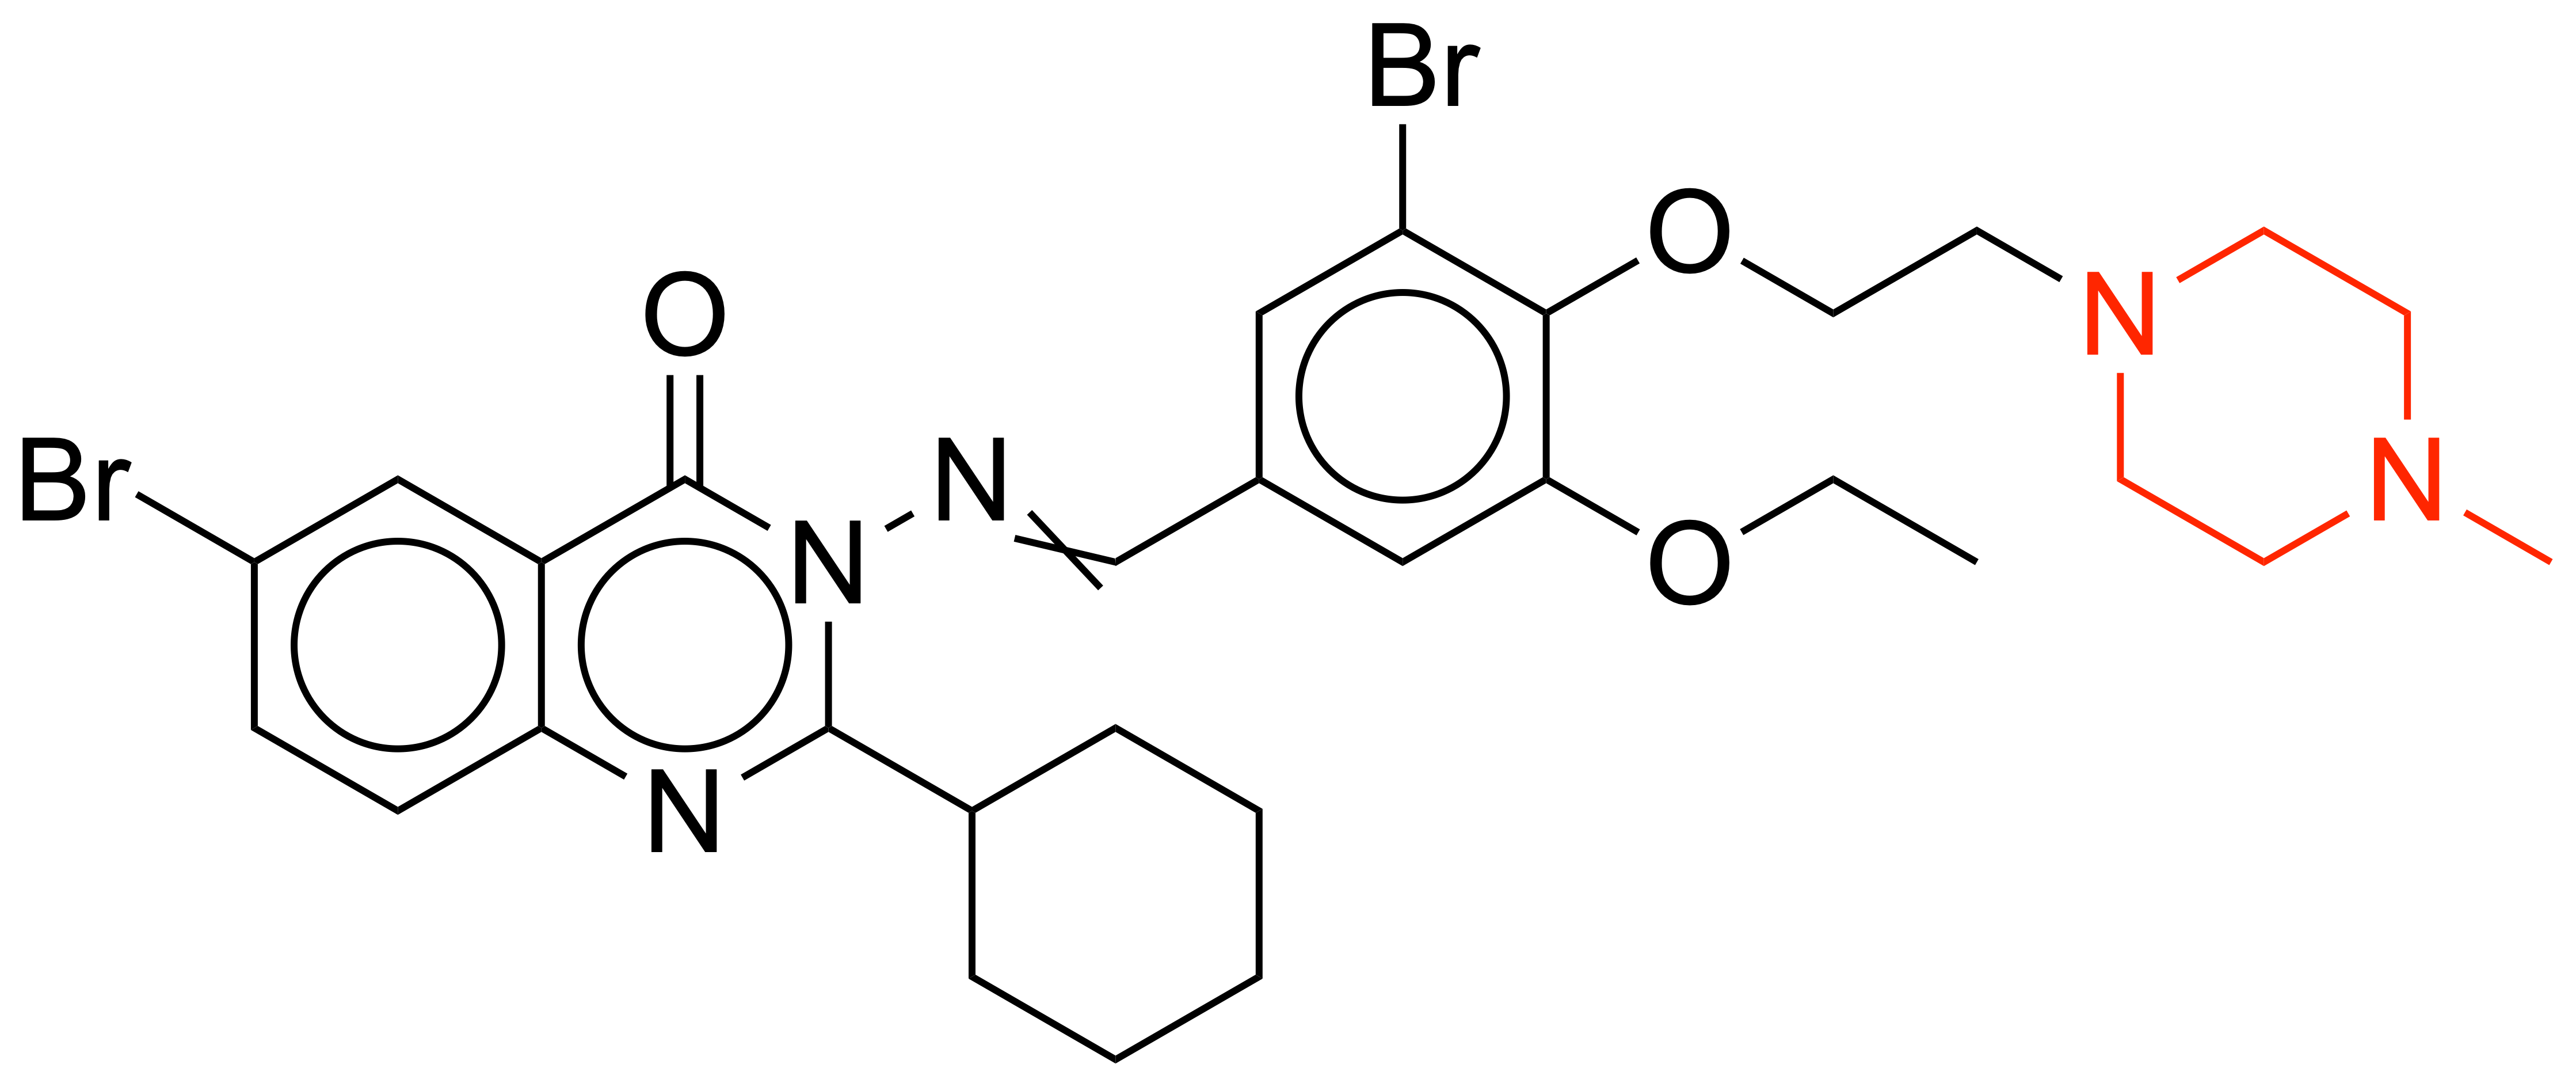}
        \par\vspace{2pt}
        \tiny BBBP=0.92 (+0.41),\\ 
        \tiny DRD2=0.47 (+0.41), QED=0.26 (+0.11)
    \end{minipage}

    \vspace{1em}

    % Second Case
    \begin{minipage}{0.43\linewidth}
        \centering
        \tiny $M_x$
        \includegraphics[width=1.0\linewidth]{./figures/BDQ_case2_mollm_src.png}
        \par\vspace{2pt}
        \tiny BBBP=0.51, \\
        \tiny DRD2=0.06, QED=0.15
    \end{minipage}
    \hfill
    \begin{minipage}{0.1\linewidth}
        \centering \Large$\Rightarrow$\\
        \raggedright \tiny \LlaSMol
        \raggedright \tiny \Sim=0.69
    \end{minipage}
    \hfill
    \begin{minipage}{0.44\linewidth}
        \centering
        \tiny $M_y$\\
        \includegraphics[width=1.0\linewidth]{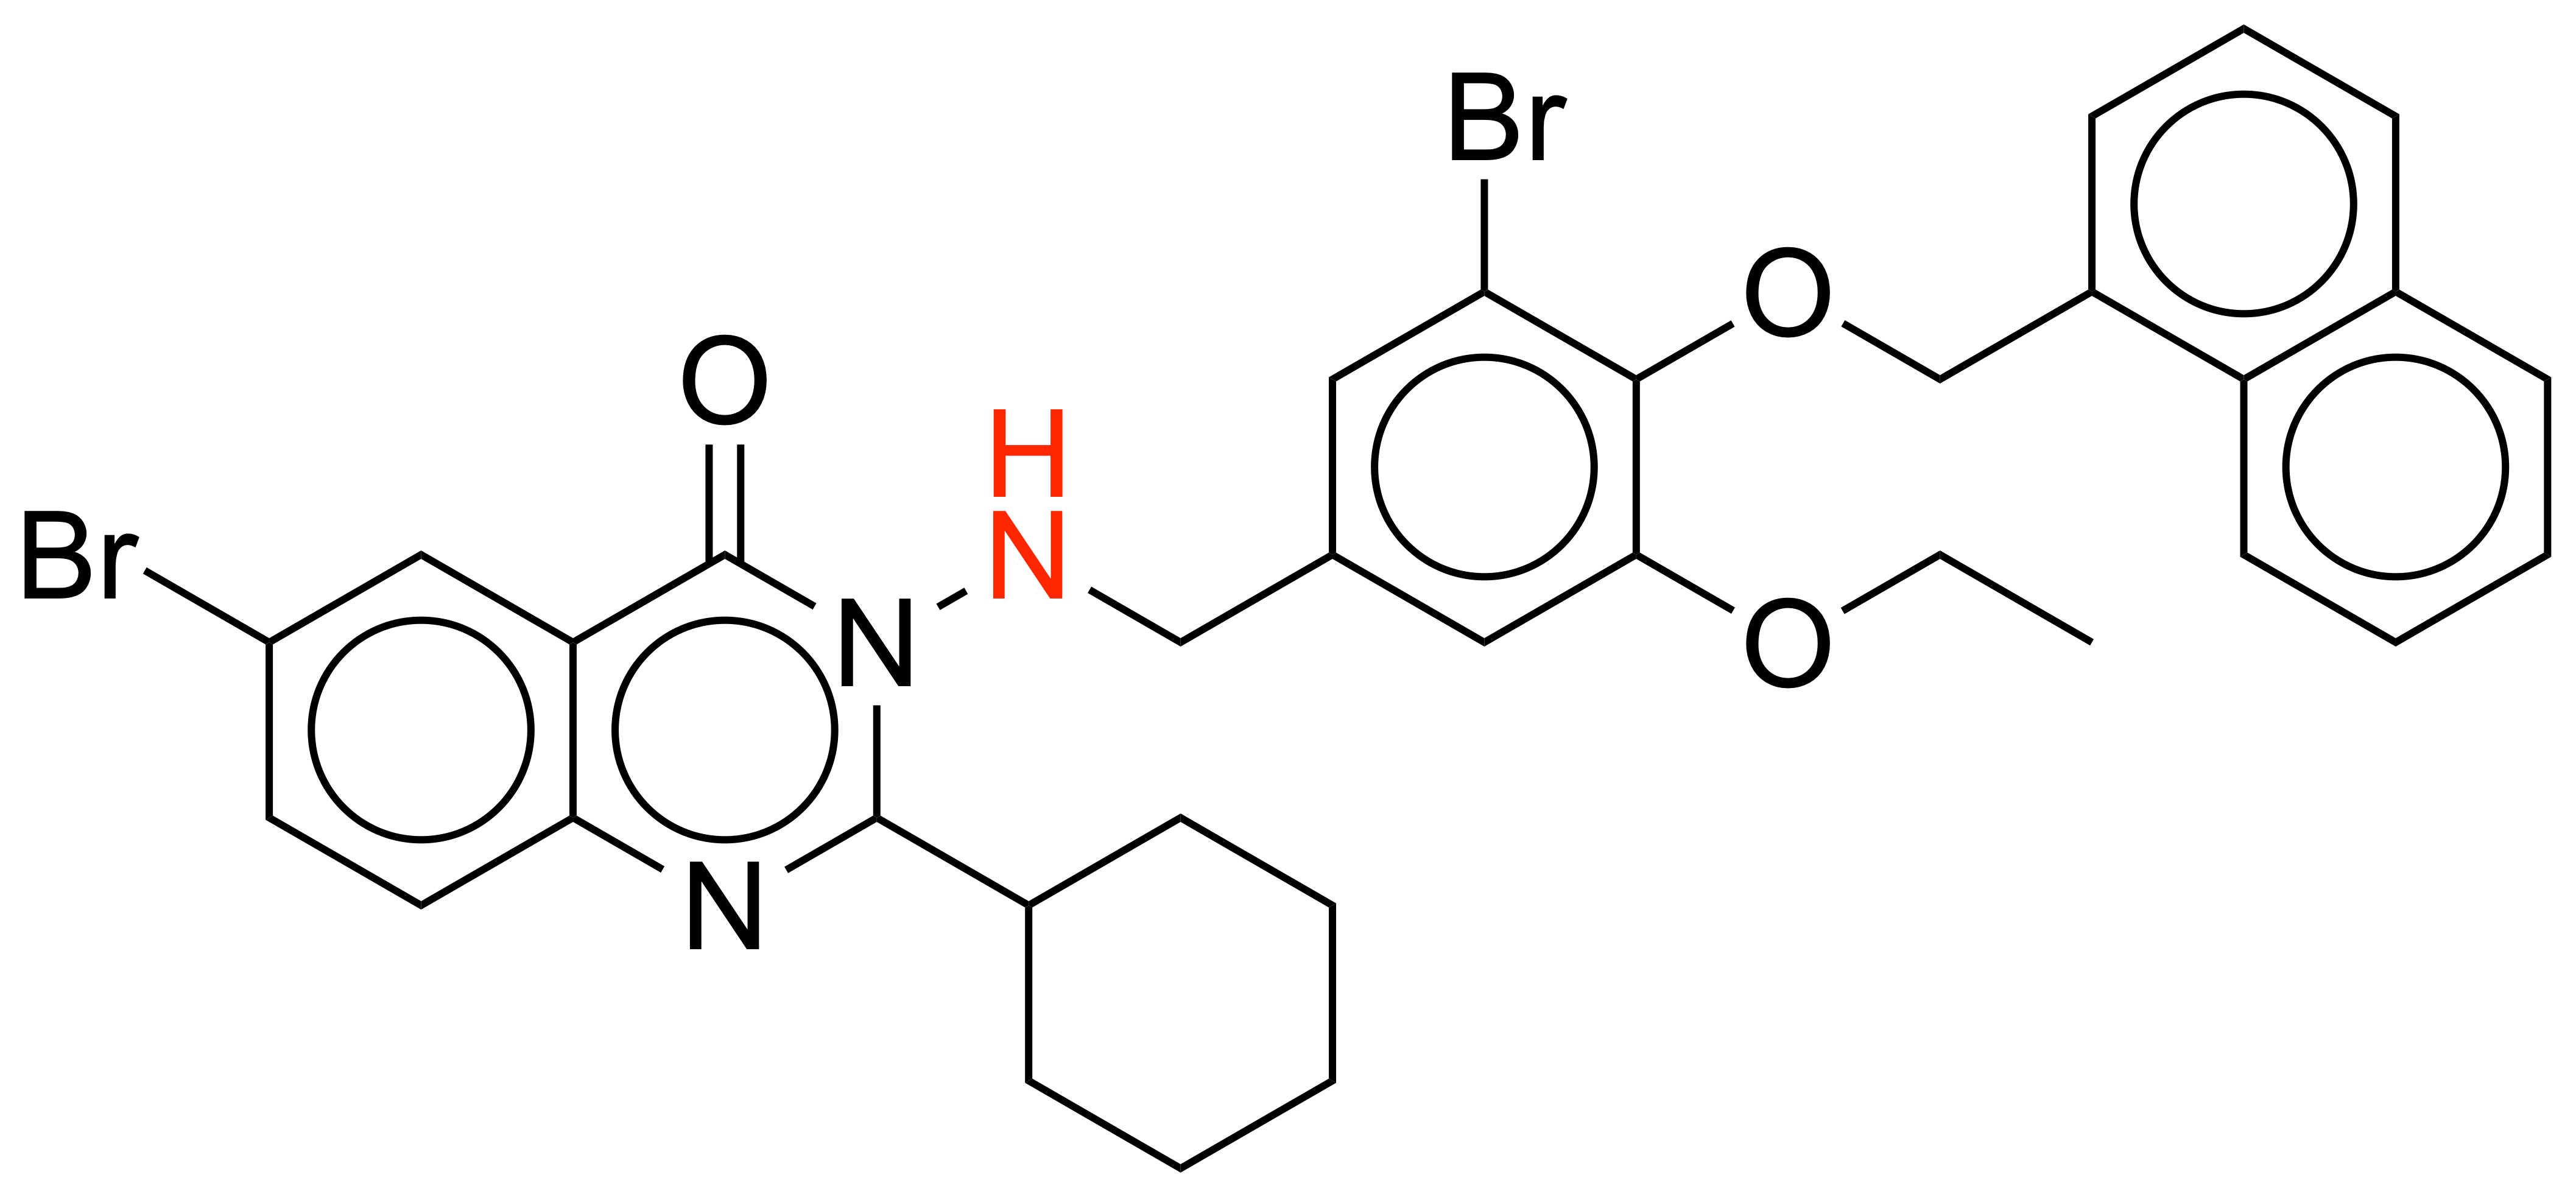}
        \par\vspace{1pt}
        \tiny BBBP=0.52 (+0.01), \\ 
        \tiny DRD2=0.07 (+0.01), QED=0.17 (+0.02)
    \end{minipage}
    %\caption{{\mollmSixGenM} and {\LlaSMolM}'s optimization case from \BDQ. Modifications are highlighted in red.}
    %\label{fig:BDQ_case2_appendix}
\end{figure}
